# Supplementary material for: Base Station Certificate and Multi-Factor Authentication for Cellular Radio Control Communication Security
Source: arXiv:2504.02133 source file (2025-04-02)
Supplement: Supplementary file 1 [file Apndx_Our_Scheme.tex]

\section{Multi-Factor Authentication Algorithm}
\label{apndx:algorithm}
\begin{algorithm}[t!]
\small
    \caption{Multi-factor authentication at user equipment using $ID,K,L,t$ \syc{lower priority}}
    \label{alg:algorithm}
    \SetKwInOut{Input}{Input}
    \SetKwInOut{Output}{Output}
    \SetKwInOut{Parameter}{Parameter}
    \Input{         $\mathcal{C}$.$ID_{i}$, $\mathcal{C}$.$K_i$, $\mathcal{C}$.$L_i$, \hfill \hfill \hfill /* \textit{Blockchain ledger} */ \\
                    \mbox{SIB1}, $ID_i$, $n$, $t$, $S_k$, \hfill \hfill \hfill /* \textit{Online communication} */ \\
                    $\bar{L}$, $\bar{t}$ \hfill \hfill \hfill /* \textit{User equipment sensing} */
                    }
    \Output{$A$ \hfill \hfill /* \textit{Authenticated? True (1), False (0)} */}
    \Parameter {$\tau_t$,$\tau_d$}
    $ A = 0$ \\
    \If{$\mathcal{C}.ID_i$ == $ID$} 
    {
       $K_i$, $L_i$ = get($ID$,$\mathcal{C}$.$K_i$, $\mathcal{C}$.$L_i$)  \\

       \If{distance($L_i$, $\bar{L}$) $\leq \tau_d$}
       {    
           % $\Delta t$ = $\bar{t} - t$ \\
       \If{($\bar{t} - t$)$ \leq \tau_t$}
            {   
                \If{$V_{K_i}$(\mbox{SIB1},$n$,$t$,$S_k$) == 1}
                {
                    \textnormal{\textbf{return}}  $ A = 1$ \hfill  \\
                }
            }
        }
    }

\end{algorithm}
\sou{Newly drafted}

The user equipment uses multiple factors ($ID, L, t, K$) from multiple sources (offline/online communication, local sensing) to yield multi-factor authentication. Algorithm~\ref{alg:algorithm} illustrates the multi-factor authentication including the sources of factors and the sequential verification. Upon successful sequential verification ensures the authenticity of the base station. 

In the offline, the blockchain ledger delivers the database, $\mathcal{C}$, containing the digital certificates of the legitimate base stations validated by the core network. Each digital certificate within $\mathcal{C}$ has base station ID, $ID$, base station public key, $K$, and the base station location, $L$. We use these three factors for authentication and we present the parameters as $\mathcal{C}.{ID}_i$, $\mathcal{C}.{K}_i$, $\mathcal{C}.{L}_i$ for any base station $i$. During online communication, i.e. SIB1 broadcast message transmission, the user equipment received SIB1, cell ID, $ID$, nonce, $n$, timestamp, $t$ and digital signature, $S_k$. During multi-factor authentication, the user equipment also senses its location, $\bar{L}$ and SIB1 reception timestamp, $\bar{t}$. The user equipment also selects two control threshold parameters $\tau_d$ and $\tau_t$ for $L$ verification and $t$ verification. All of these factors are being used in the sequential authentication verification of our scheme. The output of the sequential verification is represented by $A$ which is a boolean, where $A=0$ for not authenticated and $A=1$ is for authenticated.

At the beginning of the algorithm, the user equipment sets $A=0$, i.e. the base station is not authenticated. Then it proceeds for $ID$ verification by looking up the base station ID in the blockchain ledger, $\mathcal{C}$. If the user equipment finds a base station certificate using the cell ID ($ID$) received during the online communication then the $ID$ verification is successful and it proceeds to the $L$ verification. However, before $L$ verification, the user equipment gets the base station location, $L$, and public key, $K$ from the ledger for later verification. In $L$ verification, the user equipment measures the distance (e.g. euclidean distance) between $L$ and $\bar{L}$. If the distance is less than or equal to the threshold $\tau_d$ then the $L$ verification is successful and it proceeds to $t$ verification. In $t$ verification, the user equipment uses the timestamp, $t$, and its measured timestamp, $\bar{t}$. If $\bar{t}-t$ is less than or equal to $\tau_t$ then the $t$ verification is considered successful. Upon successful $t$ verification, the user equipment proceeds for SIB1 message verification by verifying the digital signature. In SIB1 verification, it uses $K$ received offline and $S_k$ received online. If the digital signature verification $V_{K_i}$(SIB1,$n$,$t$,$S_k$) results in $1$ then the SIB1 verification is successful. Upon successful SIB1 verification, the final algorithm output yields $A=1$, i.e. the base station is authenticated. If the verification fails at any step in the sequence then the authentication results in $A=0$, i.e. base station not authenticated.
